# Supplementary material for: Precise Fermi-level engineering in a topological Weyl semimetal via fast ion implantation
Source: arXiv:2310.07828 source file (2023-10-11)
Supplement: Supplementary file 1 [file supplementary.tex]

\documentclass{article}

\usepackage{graphicx} % Required for inserting images
\usepackage[dvipsnames]{xcolor}
\newcommand{\figref}[1]{\textcolor{blue}{Figure~\ref{#1}}}
 
\usepackage{times,xspace}
\usepackage{graphicx, graphics, color, epsfig}
\usepackage{amsmath}
\usepackage{amssymb}
\usepackage{amsfonts}
\usepackage{amsfonts}
\usepackage{epstopdf}
\usepackage[T1]{fontenc}
\usepackage{amsmath}
\usepackage{amssymb}
\usepackage{siunitx}
\usepackage{braket}
\usepackage{xcolor}
\usepackage{bbm}
\usepackage{color}
\usepackage{float}
\usepackage[colorlinks=true]{hyperref} 
\usepackage{authblk}

\title{H-TaP SI}

\date{July 2023}

\title{Precise Fermi level engineering in a topological Weyl semimetal via fast ion implantation}

\appendix
\setcounter{table}{0}

\setcounter{figure}{0}

\setcounter{equation}{0}

\section{DFT}

\textbf{Ab initio calculations:} The density functional theory (DFT) [1,2] calculations are performed using the Vienna ab initio simulation package (VASP) [3,4]. Generalized gradient approximation (GGA) in the form of Perdew-Burke-Ernzerhof (PBE) [5] is used to treat the exchange-correlation interactions. Core and valence electrons are treated by the projector augmented wave (PAW) method [6] and a plane wave basis, respectively. A tight-binding Hamiltonian is built from the DFT results using the Wannier90 package [7]. The tight-binding Hamiltonian is used to find Weyl points with the help of the WannierTools package [8]. In doped TaP, the concentration of H is around 2×10$^{21}$ cm$^{-3}$.

\section{SRIM and TRIM Calculation}
We employed the SRIM (stopping and range of ions in matter) and TRIM (transport of ions in matter) software [\textcolor{red}{cite}] to simulate realistic irradiation conditions and investigate the defect profile. TRIM simulations provided us with the flexibility to adjust parameters such as target type, thickness, and incident ion beam energy. Through the TRIM simulations, we obtained valuable results that revealed the depth profile generated by both the incident ions and recoils. For our study, we deliberately chose H$^{-}$ ions with an energy of 20 keV to irradiate the TaP crystal. This selection was driven by our specific interest in doping the ions near the surface of the sample. By considering the beam current and aperture size, we accurately calculated the incident ion flux. Furthermore, we accounted for the subtraction of secondary electrons and the total duration of irradiation, enabling us to determine the precise number of implanted ions in each sample. In our experimental setup, we utilized a 4 mm diameter beam to irradiate samples of size 2$\times$2 mm$^{2}$. The beam current for S$_{3m}$ was 140 nA, and for S$_{20m}$ and S$_{2h}$ was 170 nA. To optimize the total doping concentration as per our research interest, we varied the irradiation time accordingly.

%\section{HRTEM}

%\begin{figure}[ht!]
    %\centering
   % \includegraphics[width=1.0\columnwidth]{HRTEM.pdf}
    %\caption{\textbf{a} HAADF-TEM image }
    %\label{HRTEM}.
%\end{figure}

\section{Raman measurements}

\begin{figure}[ht!]
    \centering
    \includegraphics[width=1.0\columnwidth]{Raman.pdf}
    \caption{\textbf{a} Raman }
    \label{Raman}.
\end{figure}

We performed Raman spectroscopy measurements using a \textcolor{red}{Horiba LabRam spectrometer}. In the Raman experiments, we used an excitation wavelength of 532 nm. The incident laser was focused along the c-axis using a 50× objective lens in a backscattering configuration. Raman measurements were conducted for both the TaP and S$_{3m}$ samples. The analysis of the irradiated sample revealed peak broadening at a Raman shift of 380 cm$^{-1}$, indicating the presence of disorder within the material.

\section{Transport Measurements}
\begin{figure}[ht!]
    \centering
    \includegraphics[width=1\columnwidth]{Rxx.pdf}
    \caption{Temperature variation of longitudinal resistivity, $\rho_{xx}$ and transverse resistivity, $\rho_{xy}$, for different doping concentrations.}
    \label{Rxx}.
\end{figure}

The electrical measurements were carried out using the electrical transport option (ETO) of the physical property measurement system (PPMS). To obtain the required data, we utilized the ETO with a six-probe configuration, enabling simultaneous measurements of both $\rho_{xx}$ and $\rho_{xy}$. To minimize the influence of manually-made contact misalignment, we employed a symmetric probe configuration. In this setup, the longitudinal resistivity $\rho_{xx}$ exhibited symmetry with respect to the applied magnetic field, while the transverse resistivity $\rho_{yx}$ displayed antisymmetry. We employed the following equations to achieve this configuration:

\begin{equation}
\rho_{xx}(B) = \frac{\rho_{xx}(+B) + \rho_{xx}(-B)}{2},  
\\
\rho_{xy}(B) = \frac{\rho_{xx}(+B) - \rho_{xx}(-B)}{2}\\
\end{equation}.

The magnetic field dependence of $\rho_{xx}$ and $\rho_{xx}$ at different temperatures is illustrated in \figref{Rxx}. Shubnikov-de Haas (SdH) oscillations can be observed in both $\rho_{xx}$ and $\rho_{xx}$ at low temperatures, up to 15 K for S$_{3m}$ and 10 K for S$_{20m}$. However, no such oscillations are observed for S$_{2h}$ sample, indicating that the presence of high disorder suppresses the quantum oscillations. Thus, our further experimental analysis primarily focuses on the S$_{3m}$ and S$_{20m}$ samples, as our main interest lies in precise Fermi level engineering in a topological Weyl semimetal.

\subsection{Carier concentration and mobility}

\begin{center}
    \begin{figure}[ht!]
        \centering
        \includegraphics[width=1\columnwidth]{Sxx.pdf}
        \caption{Temperature variation of longitudinal resistivity, $\rho_{xx}$ and transverse resistivity, $\rho_{xy}$, for different doping concentrations.}
        \label{Sxx}
    \end{figure}
\end{center}

\begin{center}
    \begin{figure}[ht!]
        \centering
        \includegraphics[width=1\columnwidth]{Sxx_20.pdf}
        \caption{Temperature variation of longitudinal resistivity, $\rho_{xx}$ and transverse resistivity, $\rho_{xy}$, for different doping concentrations.}
        \label{Sxx_20}
    \end{figure}
\end{center}

To investigate the impact of irradiation on carrier concentration and mobility, we calculated the longitudinal conductivity $\sigma_{xx}$ and transverse conductivity $\sigma_{xy}$ using the following equations:

\begin{equation}
\sigma_{xx} = \frac{\rho_{xx}} {{\rho_{xx}^2 + \rho_{xy}^2}}, 
\\
\sigma_{xy} = -\frac{\rho_{xy}} {{\rho_{xx}^2 + \rho_{xy}^2}}
\end{equation}.

The field dependence of $\sigma_{xx}$ and $\sigma_{xy}$ at different temperatures is illustrated in \figref{Sxx} and \figref{Sxx_20}. To extract the carrier concentration and mobility, we simultaneously fit the $\sigma_{xx}$ and $\sigma_{xy}$ data using a two-band model defined by:

\begin{equation}
    \sigma_{xx} = \frac{n_{e}\mu_{e}e}{1+(\mu_{e}B)^2} +\frac{n_{h}\mu_{h}e}{1+(\mu_{h}B)^2}, 
    \\    
\sigma_{xy} = \left( \frac{n_{h}\mu_{h}^2}{1+(\mu_{h}B)^2} - \frac{n_{e}\mu_{e}^2}{1+(\mu_{e}B)^2} \right)eB
\end{equation}

The main text includes the temperature variation of electron and hole concentration, along with their corresponding mobility, for each doping level and compares them with pristine TaP. Our findings reveal that H$^{-}$-ion implantation significantly impacts the Fermi surface by considerably elevating the electron-hole compensation temperature despite the mobility being reduced by an order of magnitude.

\subsection{Analysis of Quantum Oscillation}
Magnetoresistance data (MR) was extracted from $\rho_{xx}$ data, using the following relation:

\begin{equation}
MR = \frac{\rho_{xx}(B) - \rho_{xx}(0)}{\rho_{xx}(0)} \times 100\%
\end{equation}

The quantum oscillation data, $\Delta$MR, was obtained by subtracting background signals from the MR data. To ensure robustness, we employed three independent methods to extract $\Delta$MR: (a) background-free curvature method (\figref{S3m_1} and \figref{S20m_1}), (b) polynomial background (main text), and (c) piecewise polynomial as background (\figref{S3m_3} and \figref{S20m_3}).

Notably, the fast Fourier transform (FFT) analysis unveiled distinct oscillation frequencies. After applying a standard signal filtering process through inverse FFT, we isolated the three oscillation components from the pristine data and determined the corresponding Landau levels (LLs). The LL index fan corresponding to the different frequencies for each fitting model has been plotted. All three methods consistently support the existence of a low-frequency carrier pocket, F$_{\alpha}$ 1.87 T - 3.94 T for S$_{3m}$ and 0.35 T - 1.14 T for S$_{20m}$. In contrast, the pristine TaP exhibits the same behavior in the range F$_{\alpha}$ 2.3 T - 4 T and F$_{\beta}$ 18 T - 19 T [\textcolor{red}{cite}].

Our comprehensive analysis confirms the presence of new oscillation frequencies, suggesting that the carrier pockets of the Weyl point can indeed reach the desired n = 0 Landau level, and additional Weyl nodes appear with H$^{-}$ ion irradiation.

\subsection{Extended Kohler’s rule of magnetoresistance}
The magnetoresistance (MR) curves do not converge onto a single curve when plotted against B/$\rho_{0}$, indicating that the MR = f(B/$\rho_{0}$) rule proposed by Kohler is not applicable to S$_{3m}$ and S$_{20m}$, as observed in our study [\textcolor{red}{cite}]. However, an intriguing observation is that all the curves in \figref{Kohler} a and b run nearly in parallel. This suggests the possibility of a single temperature-dependent multiplier affecting MR (y-axis) or B/$\rho_{0}$ (x-axis), causing them to coincide or merge into one curve. To understand this behavior further, MR curves are normalized by a scaling procedure using the T = 300 K curve and adjust the parameter n$_{T}$ individually for each curve \cite{PHY}. The outcome is clearly visible in \figref{Kohler} c and d, where all the curves seamlessly converge onto the T = 300 K curve when the data is scaled using B/$\rho_{0}$$n_{T}$. The corresponding values of n$_{T}$ for the different curves at various temperatures can be found in Fig \textcolor{red}{add fig}. This scaling procedure sheds light on the temperature-dependent behavior of the magnetoresistance and provides valuable insights into the underlying physical mechanisms governing the observed phenomena. We have further normalized n$_{T}$ and compared it with the data extracted by using a two-band model from the relation \cite{PHY}:

\begin{equation}
n_{T} = e \left[\frac{\left(\sum_{i} n_{i} \mu_{i}\right)^{3/2}}{\left(\sum_{i} n_{i} \mu_{i}^{3}\right)^{1/2}}\right]
\end{equation}

\begin{figure}[ht!]
    \centering
    \includegraphics[width=1\columnwidth]{S_3m_bckg1.pdf}
    \caption{\textbf{MR analysis using curvature-based background subtraction for S$_{3m}$}. In this approach, a second-order derivative with respect to the magnetic field B is applied to the MR data, automatically eliminating all linear, constant, and quadratic terms without the need for manual background selection. \textbf{a, b, and c,} MR data and their second derivatives with respect to B, up to B = 9 T, are presented at T = 2 K, 5 K, and 15 K, respectively. Additionally, $\Delta$MR variation with frequency, q(T), is shown for different temperatures in \textbf{d, e, and f}. \textbf{g, h, and i} display the SdH oscillation and Landau level index plot.}
    \label{S3m_1}.
\end{figure}

\begin{figure}[ht!]
    \centering
    \includegraphics[width=1.0\columnwidth]{S_20m_bckg1.pdf}
    \caption{\textbf{MR analysis using curvature-based background subtraction for S$_{20m}$}. In this approach, a second-order derivative with respect to the magnetic field B is applied to the MR data, automatically eliminating all linear, constant, and quadratic terms without the need for manual background selection. \textbf{a, b, and c} MR data and their second derivatives with respect to B, up to B = 9 T, are presented at T = 2 K, 5 K, and 15 K, respectively. Additionally, $\Delta$MR variation with frequency, q(T), is shown for different temperatures in \textbf{d, e, and f}. \textbf{g, h, and i} display the SdH oscillation and Landau level index plot.}
    \label{S20m_1}.
\end{figure}

\begin{figure}[ht!]
    \centering
    \includegraphics[width=1.0\columnwidth]{S_3m_bckg3.pdf}
    \caption{\textbf{MR analysis using piece wise polynomial background subtraction for S$_{3m}$}. \textbf{a, b, and c,} MR data and $\Delta$MR with respect to B, up to B = 9 T, are presented at T = 2 K, 5 K, and 15 K, respectively. Additionally, $\Delta$MR variation with frequency, q(T), is shown for different temperatures in \textbf{d, e, and f}. \textbf{g, h, and i} display the SdH oscillation and Landau level index plot.}
    \label{S3m_3}
\end{figure}

\begin{figure}[ht!]
    \centering
    \includegraphics[width=1.0\columnwidth]{S_20m_bckg3.pdf}
    \caption{\textbf{MR analysis using piece wise polynomial background subtraction for S$_{20m}$}. \textbf{a, b, and c,} MR data and $\Delta$MR with respect to B, up to B = 9 T, are presented at T = 2 K, 5 K, and 15 K, respectively. Additionally, $\Delta$MR variation with frequency, q(T), is shown for different temperatures in \textbf{d, e, and f}. \textbf{g, h, and i} display the SdH oscillation and Landau level index plot.}
    \label{S20m_3}.
\end{figure}

\begin{figure}[ht!]
    \centering
    \includegraphics[width=1.0\columnwidth]{Kohler.pdf}
    \caption{\textbf{a, b} Kohler’s rule plot of the data for S$_{3m}$ and S$_{20m}$ respectively. \textbf{c, d} Extended Kohler’s rule plot of the data.}
    \label{Kohler}.
\end{figure}

\begin{figure}[ht!]
    \centering
    \includegraphics[width=1.0\columnwidth]{Kohler2.pdf}
    \caption{\textbf{a, b} Kohler’s rule plot of the data for S$_{3m}$ and S$_{20m}$ respectively. \textbf{c, d} Extended Kohler’s rule plot of the data.}
    \label{Kohler2}.
\end{figure}

\newpage

\bibliography{100}

\bibitem{PHY} PHYSICAL REVIEW X 11, 041029 (2021).

\bibitem{1}	P. Hohenberg and W. Kohn, Inhomogeneous Electron Gas, Phys. Rev. 136, B864 (1964).\\

[2]	W. Kohn and L. J. Sham, Self-Consistent Equations Including Exchange and Correlation Effects, Phys. Rev. 140, A1133 (1965).\\

[3]	G. Kresse and J. Furthmüller, Efficiency of Ab-Initio Total Energy Calculations for Metals and Semiconductors Using a Plane-Wave Basis Set, Comput. Mater. Sci. 6, 15 (1996).\\

[4]	G. Kresse and J. Furthmüller, Efficient Iterative Schemes for Ab Initio Total-Energy Calculations Using a Plane-Wave Basis Set, Phys. Rev. B 54, 11169 (1996).\\

[5]	J. P. Perdew, K. Burke, and M. Ernzerhof, Generalized Gradient Approximation Made Simple, Phys. Rev. Lett. 77, 3865 (1996).\\

[6]	P. E. Blöchl, Projector Augmented-Wave Method, Phys. Rev. B 50, 17953 (1994).\\

[7]	A. A. Mostofi, J. R. Yates, G. Pizzi, Y. S. Lee, I. Souza, D. Vanderbilt, and N. Marzari, An Updated Version of Wannier90: A Tool for Obtaining Maximally-Localised Wannier Functions, Comput. Phys. Commun. 185, 2309 (2014).\\

[8]	Q. S. Wu, S. N. Zhang, H. F. Song, M. Troyer, and A. A. Soluyanov, WannierTools: An Open-Source Software Package for Novel Topological Materials, Comput. Phys. Commun. 224, 405 (2018).

\end{document}
